# Supplementary material for: Intrinsic Ferromagnetism in the Diluted Magnetic Semiconductor Co:TiO$_2$
Source: arXiv:1612.02235 source file (2016-12-07)
Supplement: Supplementary file 1 [file Co-TiO2-SupplementalMaterial-7-12-2016.pdf]

# Supplemental Material

# Intrinsic Ferromagnetism in Diluted Magnetic Semiconductor Co:$TiO_2$

H. Saadaoui[1], X. Luo[2], Z. Salman[1], X.Y. Cui[3,4], N.N. Bao[5], P. Bao[6], R.K. Zheng[6], L. Tseng[2], Y.H. Du[7], T. Prokscha[1], A. Suter[1], T. Liu[8], Y.R. Wang[2], S. Li[2], J. Ding[5], S.P. Ringer[3,4], E. Morenzoni*[1] and J.B. Yi*[2]

1. Laboratory for Muon Spin Spectroscopy, Paul Scherrer Institute, 5232 Villigen, Switzerland.
2. School of Materials Science and Engineering, University of New South Wales, Kensington, NSW 2052, Australia
3. The Australian Institute for Nanoscale Science and Technology, and School of Aerospace, Mechanical and Mechatronic Engineering, The University of Sydney, NSW 2006, Australia
4. Department of Materials Science and Engineering, National University of Singapore, 119260, Singapore
5. School of Physics, The University of Sydney, NSW 2006, Australia
6. Institute of Chemical and Engineering Science, Agency for Science, Technology and Research, 1 Pesek Road, Jurong Island, 627833, Singapore
7. ANKA, Karlsruhe Institute of Technology, 76344 Eggenstein-Leopoldshafen, Germany

*Email: elvezio.morenzoni@psi.ch and jiabao.yi@unsw.edu.au

**Thin film fabrication and characterization:**

All the films were deposited by a pulsed laser deposition (PLD) system. The targets were first prepared by mixing $CoCO_3$ and $TiO_2$ powders (Sigma-Aldrich, 99.99%) in a molar ratio of 5:95. Subsequently, the powders were sintered in a furnace at ambient atmosphere at 900 $^oC$ for 3 hrs. XRD analysis confirmed there were no Co and $CoCO_3$ phases in the powders. Then the powders were pressed into pellets and sintered in a furnace at ambient atmosphere at 1250 $^oC$ for 10 hours. The films were deposited on double side polished $LaAlO_3$ (001) single crystal substrates. All the films were deposited at 600 $^oC$ (nominal 900 $^oC$) using a KrF excimer laser operating at 248 nm and a fluence of 1.0-1.8 J $cm^{-2}$ (corresponding to deposition rate approximately 3-10 nm/min). The base pressure of the system is $10^{-8}$ torr. The oxygen partial pressure during film deposition was varied from $10^{-6}$ to $10^{-4}$ torr. The film thickness was controlled by the deposition time and measured by a profilometer. X-ray diffraction (XRD, Bruker, Advanced D8) using Cu $K_\alpha$ radiation ($\lambda$=1.5406 Å) was used for the structure and phase characterization. Energy dispersive X-ray spectroscopy (EDX) and X-ray photoelectron spectroscopy (XPS, *Kratos AXIS Ultra DLD)* is used for the composition analysis. The magnetic and transport properties were measured using a superconducting quantum interference device (SQUID, Quantum Design, MPMS, XL-7) system and a physical property measurement system (PPMS, Quantum Design, 14T). XMCD was performed at WERA beamline in ANKA, Karlsruhe Institute Technology University (KIT), Germany. The XMCD signals were measured by sample current with an applied magnetic field up to 2 Tesla.

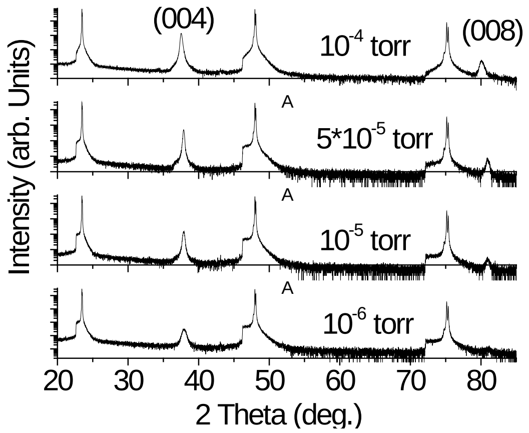


Figure S1: XRD spectra of Co-$TiO_2$ films deposited under an oxygen partial pressure of $10^{-4}$, $5*10^{-5}$, $10^{-5}$ and $10^{-6}$ torr, respectively, indicating highly texture growth.

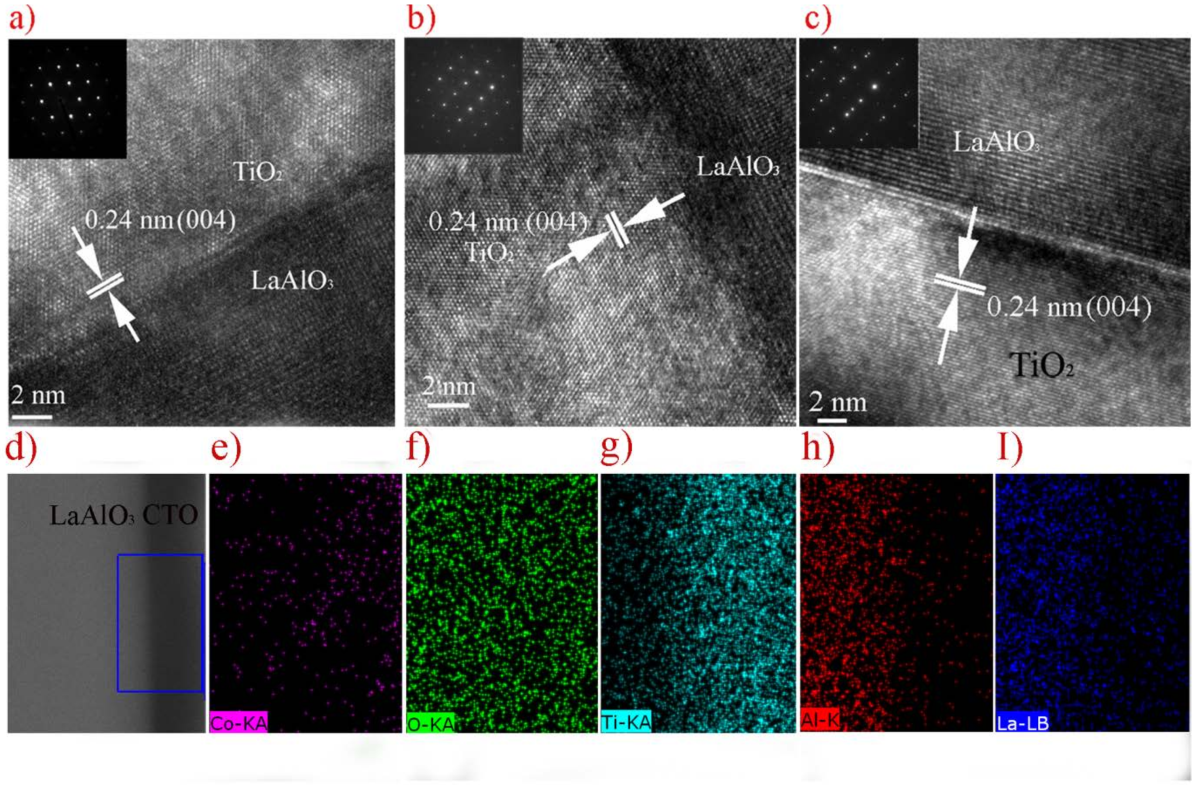


Figure S2: TEM images and EDX mapping of 5% Co doped $TiO_2$ films deposited with a deposition power of 1.8 $J/cm^2$ under different oxygen partial pressures. TEM image of a) film deposited under $10^{-4}$ torr $O_2$; b) film deposited under $10^{-5}$ torr $O_2$; c) film deposited under $10^{-6}$ torr $O_2$; d-i) Images of EDX mapping of Co, O, Ti, Al and La, respectively for the film deposited under $P_{O2}=10^{-6}$ torr.

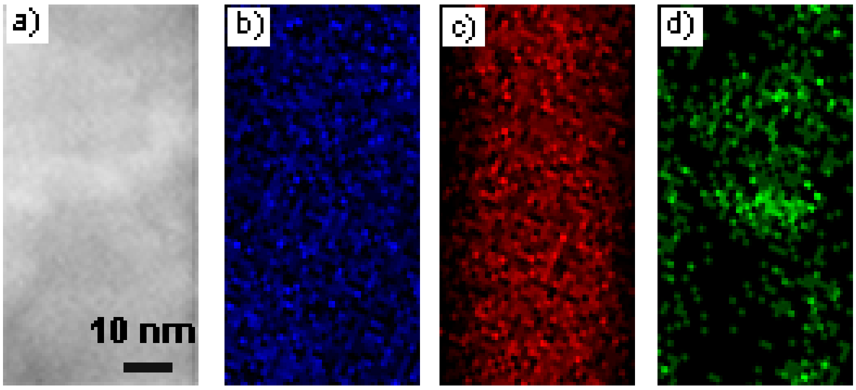


Figure S3: (a) TEM image of Co-$TiO_2$ film deposited under an oxygen partial pressure of $10^{-4}$ torr. (b), (c), (d) are the EDX mapping of the area shown in (a) for the O, Ti and Co elements respectively. A non-uniform distribution of Co atoms is observed.

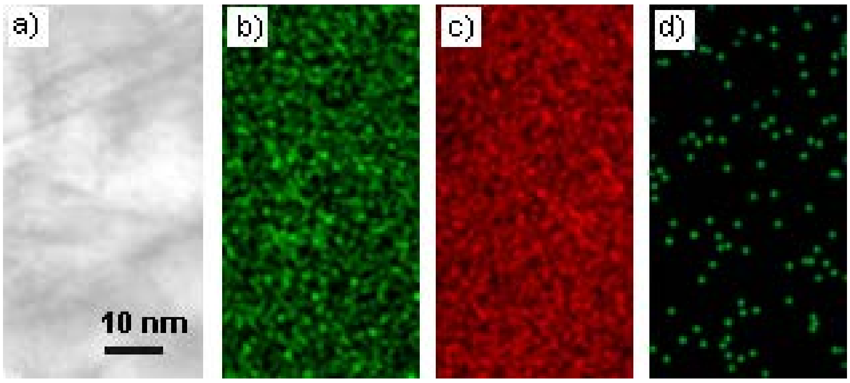


Figure S4: (a) TEM image of Co-$TiO_2$ film deposited under an oxygen partial pressure of $10^{-5}$ torr. (b), (c), (d) are the EDX mapping of the area shown in (a) for the O, Ti and Co elements, respectively.

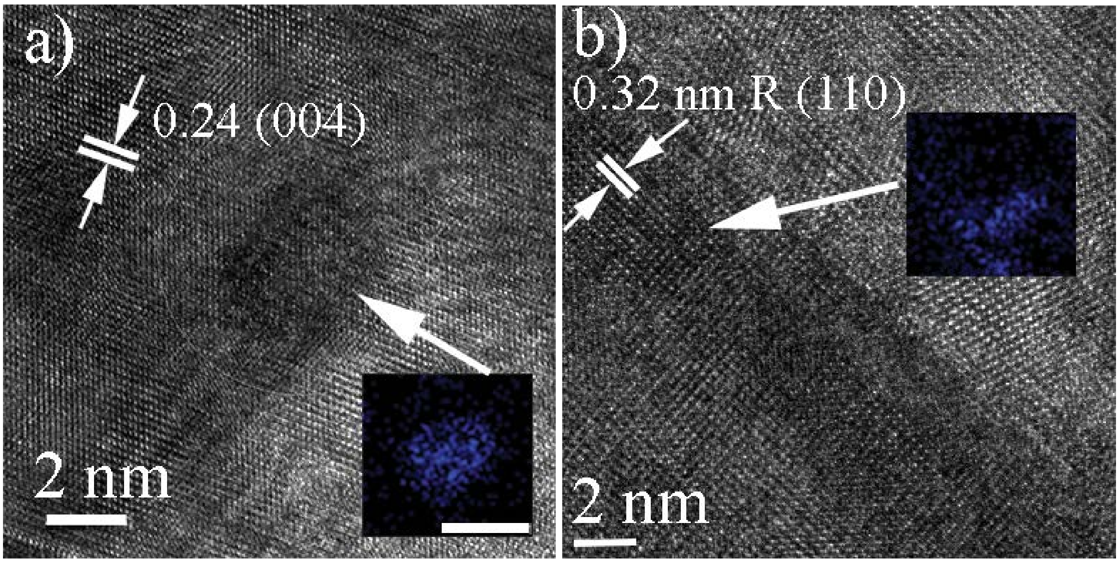

Figure S5: a) High resolution TEM images of 5% Co-$TiO_2$ deposited under an oxygen partial pressure of $10^{-5}$ torr with low deposition rate, b) the film of a) with a subsequently annealing at 600 $^{o}$C under a vacuum of $10^{-5}$ torr. The insets are corresponding EDX mapping indicating clusters formation under the two deposition conditions.

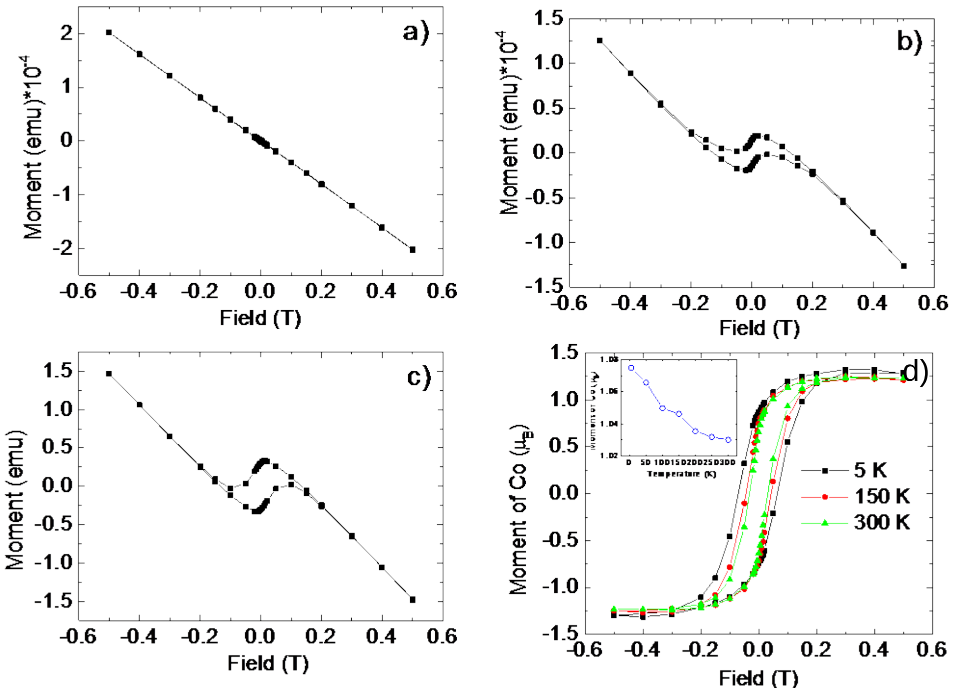


Figure S6. a), b) and c) are M-H loops of film deposited under $10^{-4}$, $10^{-5}$ and $10^{-6}$ torr $O_2$ partial pressure without subtraction of the substrate signal; d) M-H loop of the film deposited under $10^{-5}$ torr $O_2$ partial pressure taken at 300, 150 and 5 K after subtraction of the $LaAlO_3$ substrate signal. The inset is the temperature dependence of the magnetic moment.

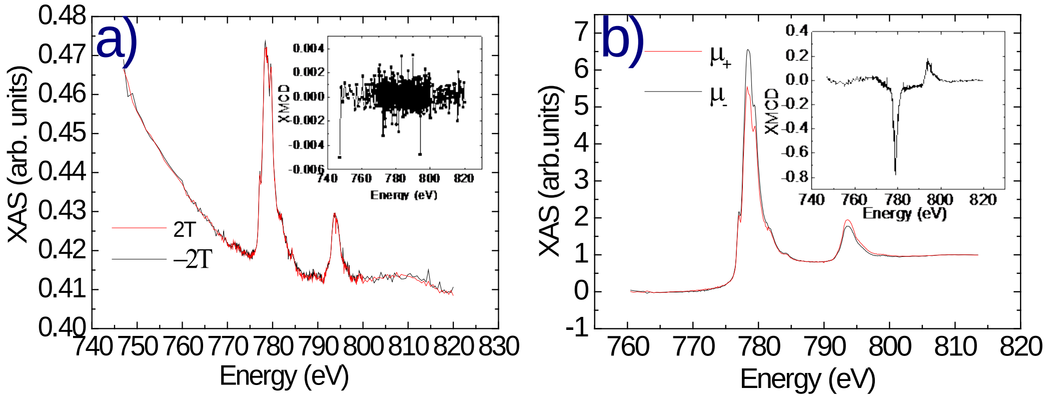

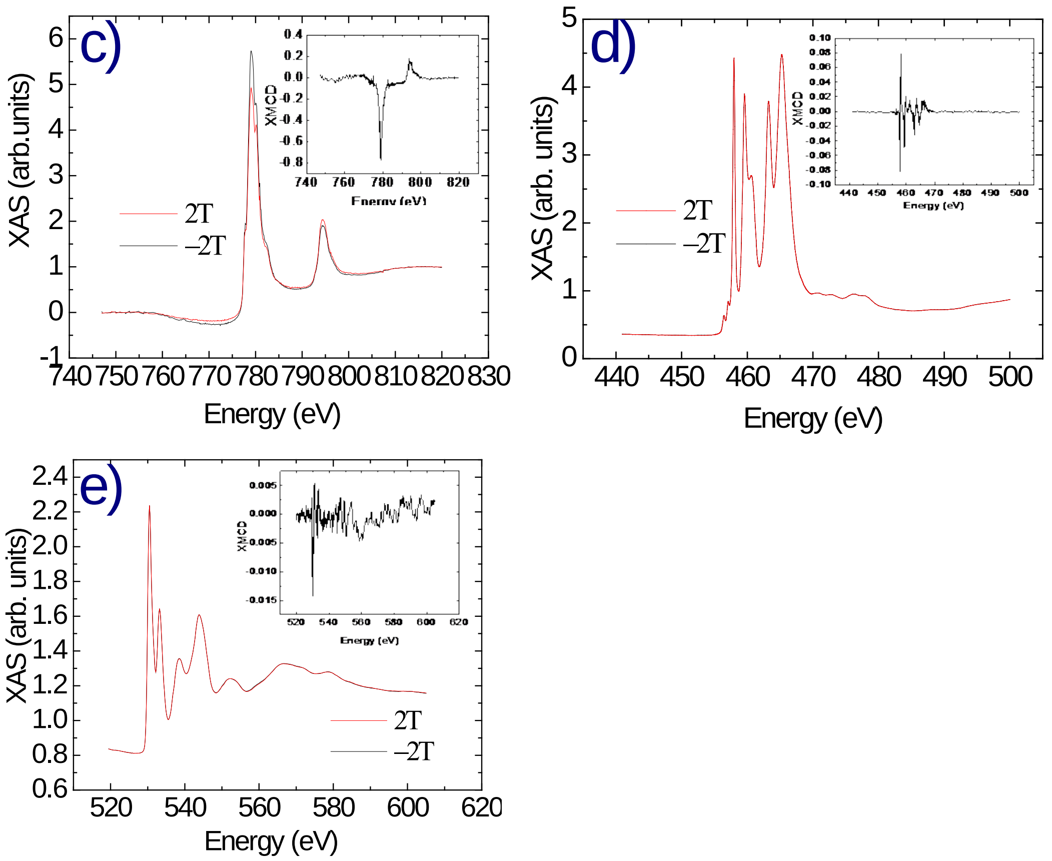


Figure S7: XAS of 5%Co-$TiO_2$ films deposited under different oxygen partial pressures. a) Co-L edge of $10^{-4}$ torr; b) Co edge of $10^{-5}$ torr; c) Co edge of $10^{-6}$ torr; d) Ti edge of $10^{-5}$ torr; e) O edge of $10^{-5}$ torr. The insets are the corresponding XMCD curves. From these graphs, it can be inferred that the magnetic moment mainly comes from Co. From the XAS and XMCD measurements of the Ti edge, small magnetic moments can be supposed. However, measurements under different magnetic fields and circular light directions indicate that the Ti ions are paramagnetic and do not contribute to the overall magnetization. The weak XMCD signal from the O edge is mostly due to noise since by changing the direction of the circular light, the XMCD curve did not change accordingly.

**μSR measurements**:

<u>Principle</u>

The μSR measurements were performed at the Low Energy Muon Instrument [1] at the μE4 beam-line [2] of the Swiss Muon Source, Paul Scherrer Institute, Switzerland. These particles are produced by moderating an intense beam of energetic ( ~ MeV) polarized muons in a moderator consisting of a condensed layer of solid Ar (~220 nm thick) capped with a thin layer of $N_2$(~10 nm). Suppression of the energy loss mechanisms responsible for the thermalization of the muon results in a high probability for the emission of epithermal muons from the moderator with a kinetic energy of about 15 eV and fully polarized [3]. These muons are accelerated to 15 keV and directed to the sample plate. The sample plate is

electrically isolated from the cold finger of the cryostat by a thick (6 mm) sapphire plate, and biased to a high voltage ranging between -12.5 to 12.5 kV. This allows changing the implantation energy of the muons between 1.5 to 26.5 keV, which corresponds to mean ranges between a few nm and ~ 200 nm. Stopping profiles as a function of muon energy are shown in Fig. S8.

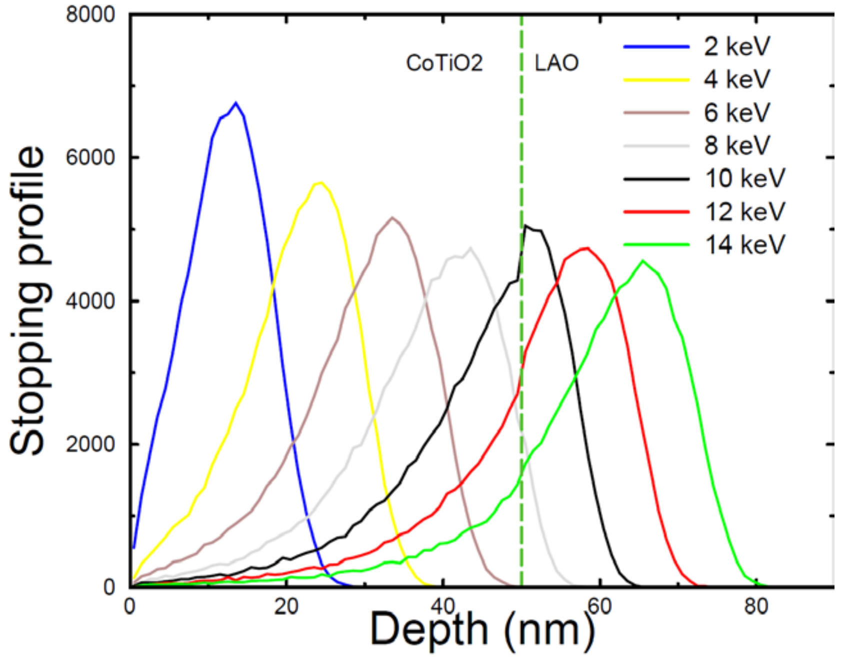


Fig. S8: Muon stopping profiles as a function of implantation energy in the 50 nm Co doped $TiO_2$ sample grown on a $LaAlO_3$ substrate. The profiles have been calculated with the TRIM.SP program adapted to simulate the muon implantation [4,5].

The LE-μSR measurements were performed in a temperature range from 5 to 300 K, in zero field with stray magnetic fields at the sample position reduced to less than 0.008 mT in all directions. Small magnetic fields can be applied perpendicular to both the initial muon spin polarization and beam direction, but parallel to the face of the substrates. The samples with a size of 2×2 cm were mounted on the Ni holder, which very quickly depolarize the muons missing the sample (about 20%) and does not produce a sizable signal. A schematic layout of the apparatus can be found in [1].

The measurements reported here were performed in a transverse magnetic field (TF) applied perpendicular to the initial muon spin polarization and to the substrate surface, or in zero external magnetic field (ZF). TF measurements are used to determine the magnetic fraction as a function of temperature.

In a μSR experiment, one is interested in the time evolution of the muon spin polarization P(t). This is determined via detection of positrons, emitted during the muon decay (lifetime $\tau_\mu$=2.197 μs), preferentially in the direction of the muon spin at the moment of decay. The number of positrons detected by a counter as a function of time after implantation reflects the time dependence of the muon spin polarization along the axis of observation defined by the detector: $N(t) = N_0(1 + AP(t))e^{-t/\tau_\mu} + N_{Bg}$, where $N_0$ is a normalization constant, A is the effective setup-dependent maximum asymmetry, and $N_{Bg}$ is a small (about 5%) time-independent random background.

The time evolution of the spin polarization is presented experimentally as an asymmetry of two positron counters located on the left (L) and right (R) (or top and bottom) to the sample sitting at the center of a cryostat;

$$A(t) \equiv AP(t) = \frac{N_R(t) - N_L(t)}{N_R(t) + N_L(t)}$$

Experimentally, one measures the projection of the spin polarization along a direction defined by the positron counters. The spin polarization depends on the static and fluctuating components of the internal magnetic field at the muon stopping site. The muon spin precesses with a characteristic Larmor frequency $\omega_L = \gamma_\mu B$, where $\gamma_\mu/2\pi$ = 135.5 MHz/T is the muon gyromagnetic ratio and B is the total magnetic field at the muon site. Therefore, in μSR one measures the local magnetic field distribution in the material. In a paramagnetic environment, P(t) is slowly-relaxing in ZF and shows a precession frequency at $\omega_L = \gamma_\mu B_{ext}$ in an external field $B_{ext}$ applied perpendicular to the initial polarization direction (so called TF geometry). In a magnetic environment, well defined precession frequencies may be observed in ZF in a static long-range ferromagnet or antiferromagnet, or a distribution of precession frequencies with the corresponding width proportional to the field inhomogeneity. If the field distribution is broad when averaged over the sample, as in the case of disordered or short range magnetism, P(t) decays with a fast relaxation. In the case of different magnetic environments, P(t) is the superposition of the corresponding magnetic and paramagnetic signals, therefore one is able to determine the magnetic and non-magnetic volume fractions.

Fitting the μSR spectra:

The TF data can be well fitted using the MusrFit package to a cosine function multiplied by an exponential taking into account the field inhomogeneities with a damping rate $\lambda_s$ [6]:

$$A(t) = Acos(\gamma_\mu Bt + \phi)e^{-\lambda_s t}$$

The amplitude of the precessing signal is a measure of the non-magnetic volume fraction. By comparing this quantity to the asymmetry in a non-magnetic sample of similar geometry, we can deduce the magnetic volume fraction of the films.

The samples grown at low pressures $P_{O2}=10^{-5}$ and $10^{-6}$ torr do not show any spontaneous precession in ZF and are fitted by a static Lorentzian Kubo-Toyabe (KT) function multiplied by an exponential

$$A(t) = A\left\{\frac{1}{3} + \frac{2}{3}(1 - \Delta t)e^{-\Delta t}\right\}e^{-\lambda_e t}$$

Here $\Delta$ is related to the width of the local field distribution by $\Delta = \gamma_\mu \Delta B$ and is proportional to the internal magnetization, and $\lambda_e$ is an additional small damping rate due to some slow electronic dynamics. The KT function is appropriate for μSR signal of randomly distributed diluted static magnetic moments. The signal in weakly magnetic samples grown at $P_{O2}=5\cdot 10^{-5}$ and $10^{-4}$ torr is better accounted for using a simple fast-relaxing exponential plus a slowly-relaxing exponential function $\lambda_s \approx 0.2(1)\mu s^{-1}$:

$$A(t) = A_f e^{-\lambda_f t} + A_s e^{-\lambda_s t}$$

The slow-relaxing component represents a combination of the paramagnetic and background signal, and the component of the magnetic signal corresponding to the first term of the KT expression. To first order in $\Delta t$, the KT function can be approximated as $1 - (4/3)\Delta t + .....$ When this is compared to the exponential decay used in the fitting $1 - \lambda_f t + ...$ , one notes that the depolarization rate of the fast component $\lambda_f$ is related to $\Delta$ by $\lambda_f \approx \frac{4}{3}\Delta$, which is the conversion factor used in Fig. 3b of the manuscript.

**First principles calculations:**

To understand the underlying mechanism of the dopant distribution and the origin of the observed ferromagnetism in Co doped $TiO_2$, we have performed extensive first principles density functional theory (DFT) calculations within the generalized gradient approximation [7] with an on-site Coulomb repulsion of U = 6.8 eV for Ti 3*d* orbitals and U = 6.5 eV for Co 3d orbitals [8] (GGA+U). The projector augmented wave pseudopotentials [9] are employed to describe the electron-ion interaction. The plane wave cut-off energy was 500 eV. The

tetrahedron method with a 5×5×4 k-mesh grid was employed for the integration in Brillouin zone. The accuracy of the electronic iterations was up to $10^{-6}$ eV. The structures were relaxed using a conjugate gradient minimization algorithm until the magnitude of residual Hellman–Feynman force on each atom was less than 0.025 eV/Å. The calculated indirect band gap value is 3.05 eV at Γ, in good agreement with the experimental value, 3.2 eV. The equilibrium bulk lattice parameters of anatase $TiO_2$ $a = b = 3.893$ Å and $c = 9.532$ Å, were found to be in good agreement with experiments ($a = b = 3.784$ Å and $c = 9.514$ Å).

We calculate the formation energy of isolated defects, including substitutional $Co_{Ti}$, interstitials $Ti_{int}$ and $Co_{int}$, O vacancy $O_{vac}$, and $Co_{Ti}$+$V_O$ complexes for neutral and charged states to determine the relative stability of the different configurations [10,11,12]. The formation energy for a charged state q for a given configuration is calculated as:

$$E^f = E_{def:TiO2} - E_{ref\text{-}TiO2} - n\,\mu_{Co} + m\,\mu_{Ti} + l\,\mu_O + q(E_F + E_v + \Delta V)$$

Where $E_{def:TiO2}$ and $E_{ref\text{-}TiO2}$ are the total energy of defective $TiO_2$ and defect-free $TiO_2$ supercell, respectively. $\mu_{Co}$, $\mu_{Ti}$, and $\mu_O$ are the atomic chemical potential of Co, Ti and O, while the integer n, m and l are the numbers of doped Co, substituted Ti and removed O atoms, respectively. $E_F$ is the Fermi level, referenced to the valence-band maximum (VBM) in bulk $TiO_2$, and varies up to the experimental bang gap value of 3.2 eV. $E_v$ is the bulk VMB of the reference $TiO_2$ supercell. The correction term ΔV is used to align the reference electrostatic potential between the supercell containing the charged defect and the bulk supercell. The defect charge-state transition level ε(q/q') is defined as the crossing-point where $E^f(q)=E^f(q')$.

**Table I:** Isosurface plots of the spin density of various stable configurations in Co doped $TiO_2$. The atomic magnetic moment (MM) and total MM values are also given. The isosurface value is 0.015 electron/Å$^3$.

| Spin Density Isosurface Plots | Description |
| --- | --- |
| (a): $(Co_{Ti})^0$ 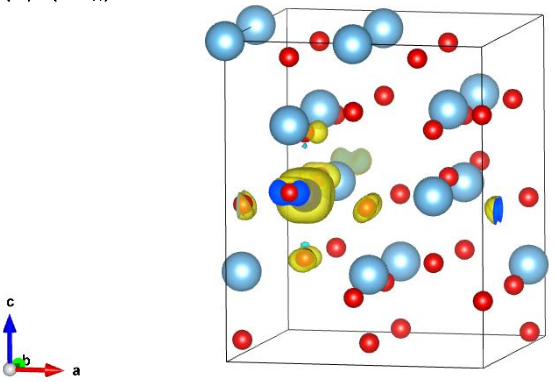 | Single neutral Co substitution on Co:<br>MM on Co: 0.71 $\mu_B$<br>MM on O: 0.033 $\mu_B$<br>MM on Ti: 0.001 $\mu_B$<br>Total MM per cell: 0.93 $\mu_B$ |
| (b): $(Co_{Ti})^{2-}$ 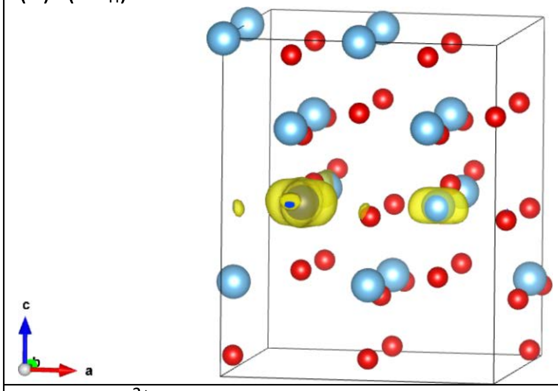 | Single charged substitutional Co:<br>MM on Co: 0.75 $\mu_B$<br>MM on O: 0.001 $\mu_B$<br>MM on Ti: 0.1 $\mu_B$<br>Total MM per cell: 0.99 $\mu_B$ |
| (c): $(Co_{int})^{2+}$ 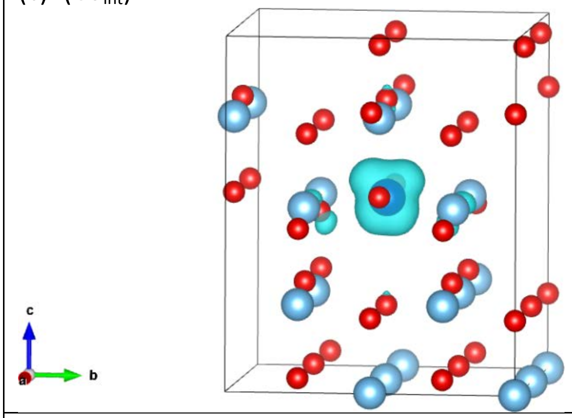 | Single charged Co interstitial dopant:<br>MM on Co: 0.92 $\mu_B$<br>MM on O: 0.01 $\mu_B$<br>MM on Ti: 0.01 $\mu_B$<br>Total MM per cell: 0.96 $\mu_B$ |
| | Single charged O vacancy<br>Non-magnetic |

| | |
|---|---|
| (d): $V_O^{2+}$ 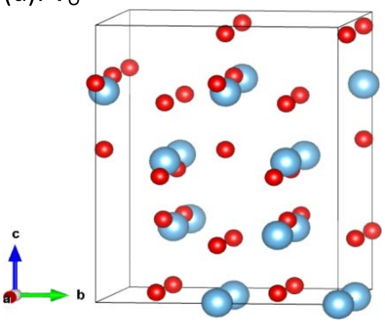 | |
| (e): $Ti_{int}^{4+}$ 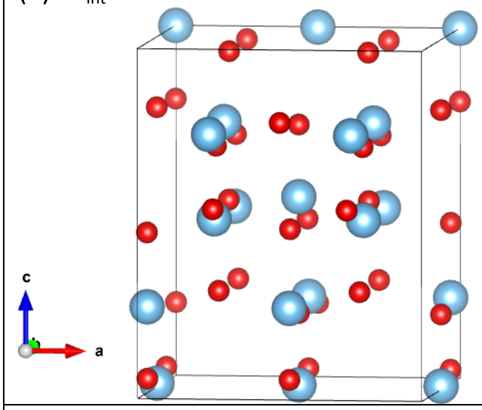 | Single charged Ti interstitial defect<br><br>Non-magnetic |
| | |
| (f) $(Co_{Ti}V_O)^0$ 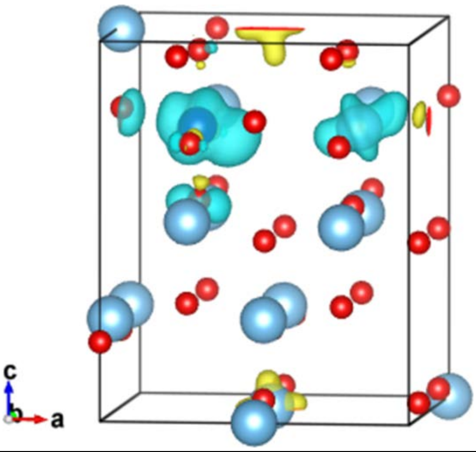 | Neutral $Co_{Ti}$ + $V_O$ complex<br><br>MM on Co: 0.86 $\mu_B$<br><br>MM on O: 0.005 $\mu_B$<br><br>MM on Ti: one 0.1 $\mu_B$<br><br>Total MM per cell: 0.95 $\mu_B$ |
| (g) $(Co_{Ti}V_O)^{+1}$ 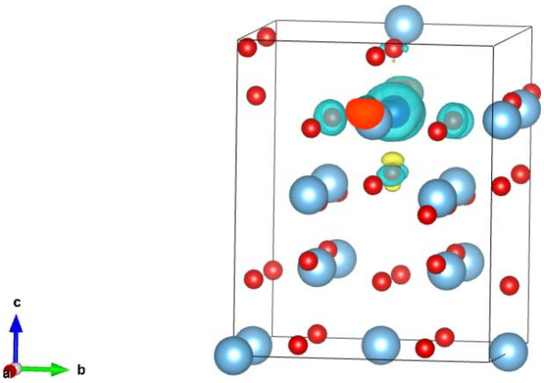 | Charged $Co_{Ti}$ + $V_O$ complex<br><br>MM on Co: 1.51 $\mu_B$<br><br>MM on O: 0.09 $\mu_B$<br><br>MM on Ti: one 0.1 $\mu_B$<br><br>Total MM per cell: 1.89 $\mu_B$ |
| (h) pair-$Co_{Ti}$ | Neutral pair $Co_{Ti}$ at the nearest config.<br>Co-Co couples ferromagnetically |

| | |
|---|---|
| 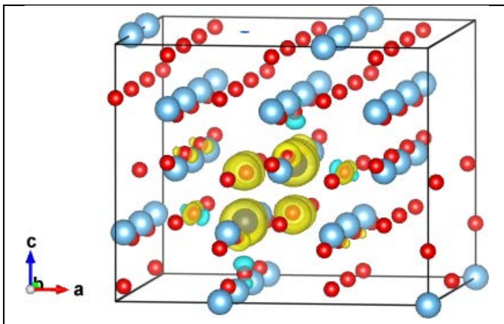<br> | MM on Co: 0.67 $\mu_B$<br><br>MM on two O: 0.2 $\mu_B$<br><br>MM on Ti: one 0.008 $\mu_B$<br><br>Total MM per cell: 1.89 $\mu_B$ |
| (h) triple-$Co_{Ti}$<br>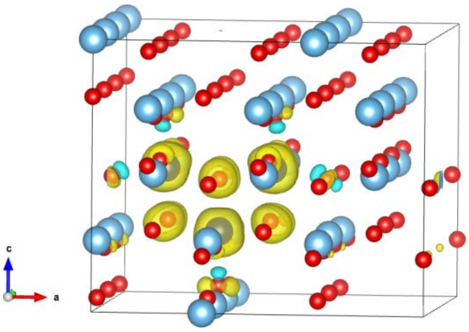 | Neutral triple $Co_{Ti}$ clusters at the nearest config.<br>Co-Co couples ferromagnetically<br>MM on Co: 0.64 x2; 0.72 $\mu_{B,}$<br><br>MM on two O: 0.24 x3 $\mu_B$<br><br>MM on Ti: one 0.008 $\mu_B$<br><br>Total MM per cell: 2.8 $\mu_B$ |
| (i)4-$Co_{Ti}$<br>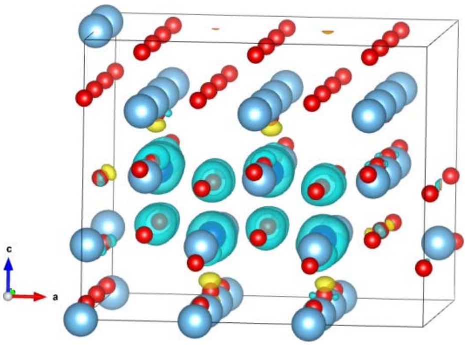 | Neutral four-$Co_{Ti}$ clusters at the nearest config.<br>Co-Co couples ferromagnetically<br>MM on Co: 0.62 x2; 0.70 x2 $\mu_{B,}$<br><br>MM on two O: 0.24 x 4 $\mu_B$<br><br>MM on Ti: one 0.007 $\mu_B$<br><br>Total MM per cell: 3.73 $\mu_B$ |
| (j)pair $(Co_{Ti}+V_O)^0$-near<br>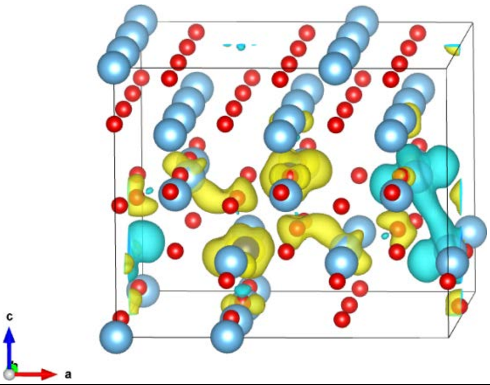<br> | Neutral pair ($Co_{Ti}$+$V_O$) at the near config.<br><br>MM on Co: 1.2 $\mu_{B,}$<br><br>MM on two O: 0.1 x 4 $\mu_B$<br><br>MM on Ti: -0.59 x 2 $\mu_B$<br><br>Total MM per cell: 1.90 $\mu_B$ |
| (k)pair $(Co_{Ti}+V_O)^{+2}$-near | Charged pair ($Co_{Ti}$+$V_O$) at the near config.<br><br>MM on Co: 1.5 $\mu_{B,}$<br><br>MM on two O: 0.1 x 4 $\mu_B$<br><br>MM on Ti: 0.15 x 2 $\mu_B$ |

| | |
|---|---|
| 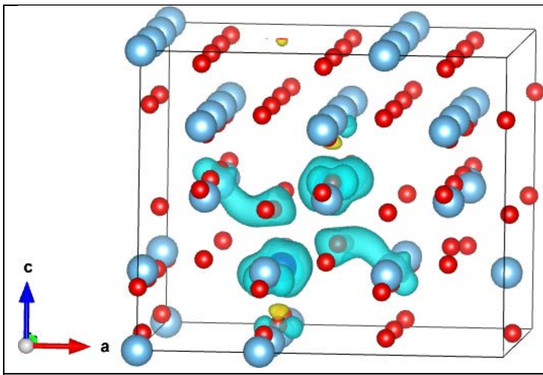  | Total MM per cell: 3.8 $\mu_B$ |
| (l) pair $(Co_{Ti}+V_O)^0$-far 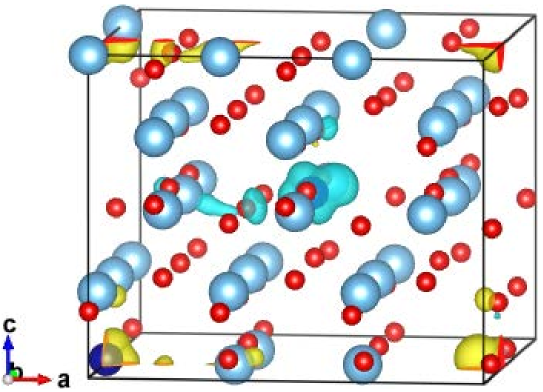  | Neutral pair $(Co_{Ti}+V_O)$ at the seperated config.<br><br>Very weak antiferromagnetic (~5 meV) over FM<br><br>MM on Co: +/-0.87 $\mu_{B,}$<br><br>MM on two O: +/-0.05 $\mu_B$<br><br>MM on Ti: +/-0.07 $\mu_B$<br><br>Total MM per cell: 0 μ |
| (m) $(Co_{Ti}+V_O)^{+2}$-medium 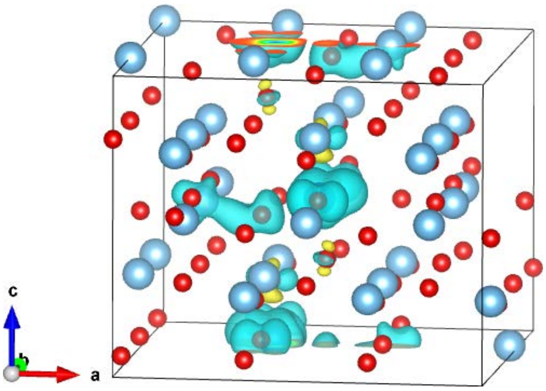  | Charged pair $(Co_{Ti}+V_O)$ with a medium separation<br><br>Rather weak ferromagnetic (~11 meV) over AFM<br><br>MM on Co: 1.5 $\mu_{B,}$<br><br>MM on two O: 0.1 x 4 $\mu_B$<br><br>MM on Ti: 0.15 x 2 $\mu_B$<br><br>Total MM per cell: 3.8 $\mu_B$ |

a)

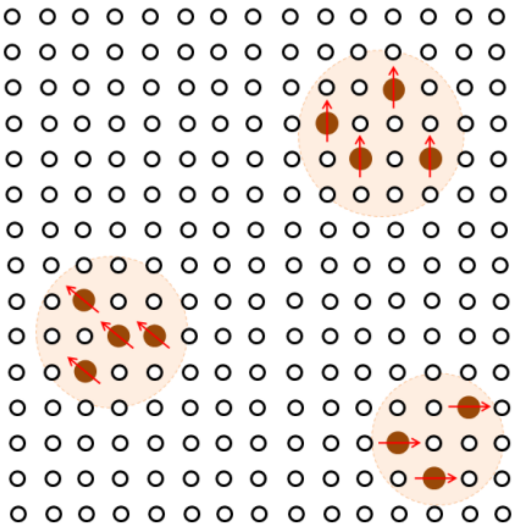

b)

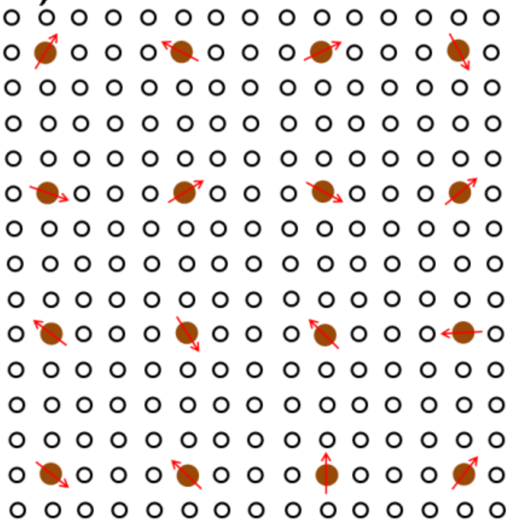

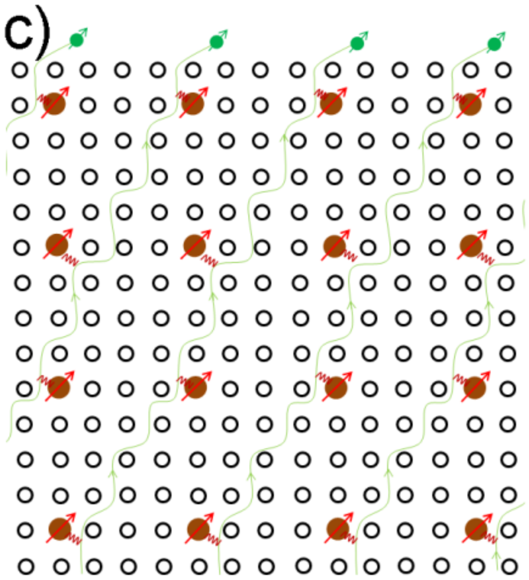


Figure S9: Description of three models for the explanation of magnetic phenomena in Co-doped $TiO_2$ films. (a) Formation of isolated magnetic polarons in the film deposited under high oxygen partial pressure, resulting in paramagnetism at room temperature and ferromagnetic ordering at low temperature ($PO_2=10^{-4}$ torr). (b) Uniform distribution of magnetic dopants without sufficient carrier mediation, leading to paramagnetism or very weak ferromagnetism ($PO_2=5*10^{-5}$ torr). (c) Uniform distribution of magnetic dopants with sufficient carrier mediation, leading to ferromagnetic ordering ($PO_2=10^{-5}$ torr and $10^{-6}$ torr ).

References:

[1] E. Morenzoni, H. Glückler, T. Prokscha, H. P. Weber, E. M. Forgan, T. J. Jackson, H. Luetkens, C. Niedermayer, M. Pleines, M. Birke, A. Hofer, J. Litterst, T. Riseman and G. Schatz, Physica B 289, 653 (2000).
[2] T. Prokscha, E. Morenzoni, K. Deiters, F. Foroughi, D. George, R. Kobler, A. Suter and V. Vrankovic, Nuclear Instruments and Methods in Physics Research A 595, 317 (2008)
[3] E. Morenzoni, F. Kottmann, D. Maden, B. Matthias, M. Meyberg, T. Prokscha, T. Wutzke and U. Zimmermann, Phys Rev Lett 72, 2793 (1994).
[4] D. Eckstein, Computer Simulation of Ion-Solid Interactions. (Springer, Berlin, Heidelberg, New York, 1991).
[5] E. Morenzoni et al., Nuclear Instr. and Meth. in Phys.Res. B 192 254 (2002).
[6] A. Suter, B. M. Wojek, Phys. Procedia 30, 69–73 (2012).
[7] G. Kresse and D. Joubert, Computational Materials Science 6, 15 (1996).
[8] V. I. Anisimov, J. Zaanen, and O. K. Anderson, Phys. Rev. B 44, 943 (1991).
[9] G. Kresse and D. Joubert, Phys. Rev. B 59, 1758 (1999).
[10] C. G. Van de Walle and J. Neugebauer, J. Appl. Phys. **95**, 3851 (2004).
[11] X. Y. Cui, B. Delley, A. J. Freeman and C. Stamplfl, Phys. Rev. B 76, 045201 (2007).
[12] H. Kizaki, M. Toyoda, K. Sato, and H. Katayama-Yoshida, Applied Physics Express 2 053004 (2009).
